# Supplementary material for: Quantum echo route towards exceptional points in Anderson localized lasers
Source: arXiv:2301.06532 source file (2023-01-16)
Supplement: Supplementary file 1 [file Supplementary_draft_new.pdf]

# Supplementary information for Quantum echo route towards exceptional points in Anderson localized lasers

Krishna Joshi and Sushil Mujumdar

*Nano-optics and Mesoscopic Optics Laboratory, Tata Institute of Fundamental Research,*

*1<sup>st</sup> Homi Bhabha Road, Mumbai, 400 005, India*

## **Coupled ring resonator simulation using the eigenvalue solver based on Finite Element Method (COMSOL Multiphysics):**

**Figure S1(a)** depicts a coupled micro-ring resonator arrangement (radius = 2  $\mu\text{m}$  and thickness = 0.2  $\mu\text{m}$ ) with gains or loss represented by  $g_i$  ( $i = 1, 2$ ) and coupling strength ( $\kappa$ ). The coupling strength determines the mutual overlap of their respective modal fields. This model was simulated in COMSOL using the Finite Element Method (FEM).

**Figure S1(b)** demonstrates the calculated complex eigenfrequencies and corresponding field distributions in both cavities above and below the exceptional point (EP). Clearly, when both rings are subjected to the same level of gain [starting point of the subplot plot (b)], the frequency splitting in real part is large while their imaginary part remains degenerate. Their field profiles [shown in subplot (b) insets] exhibit bonding (upper branch) and anti-bonding (lower branch) behaviour, with an even distribution of eigenmodes between the rings. As gain in the 2<sup>nd</sup> cavity is gradually reduced while the gain in the first cavity remains constant, the splitting in real eigenfrequency decreases until the system reaches the exceptional point (EP) at which eigenfrequencies become completely identical in both their real and imaginary parts. Beyond this point, the real eigenfrequencies degenerate, while the imaginary part splits

into two branches, corresponding to the broken PT symmetry regime. In this regime, the eigenmodes reside only in one of the cavities and named as amplifying and decaying modes, as shown in the insets of subplot (b).

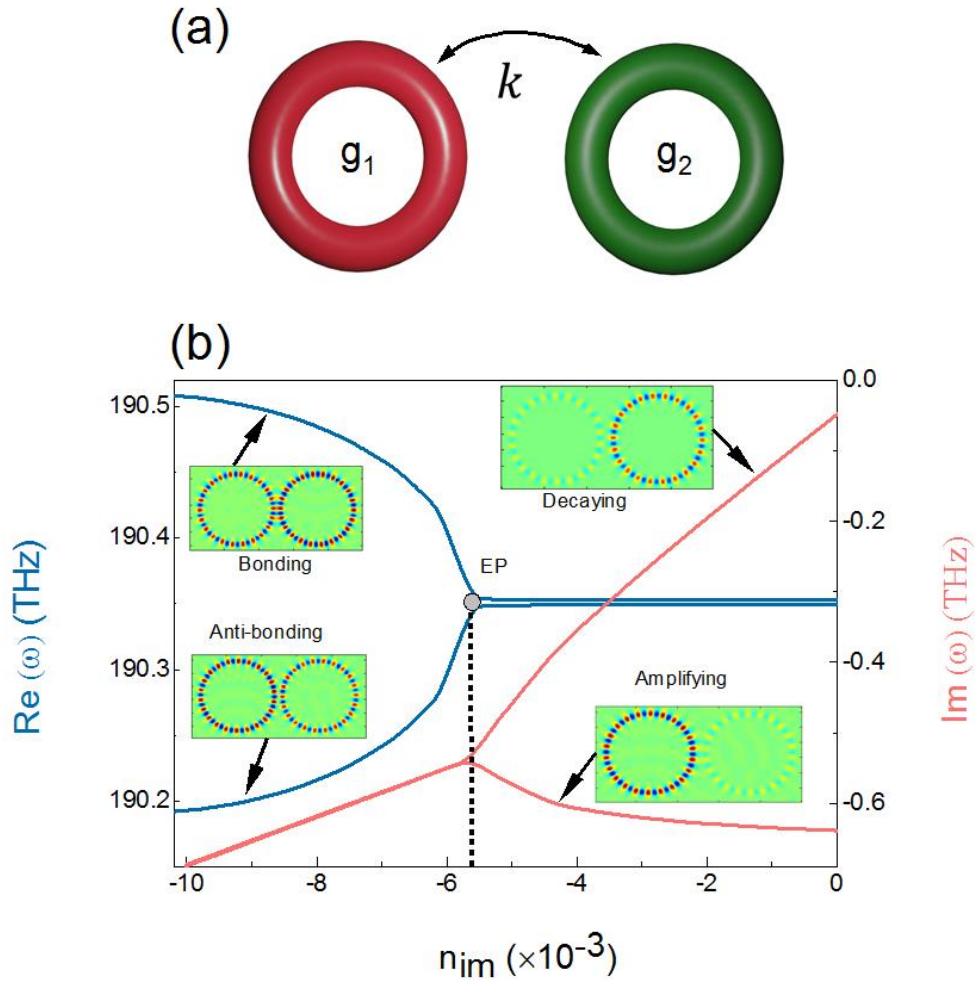

**Figure S1. (a) Schematic of the** coupled ring resonator with gain  $g_i$  ( $i = 1, 2$ ) and coupling strength  $\kappa$ . (b) Computed eigenfrequencies and corresponding eigenmodes (insets) in approach to EP.

## **Spectral mode analysis of Isolated modes and Exceptional points (EPs):**

In order to study the spectral response, the output lasing emission spectra were fitted with the Lorentzian  $L(\omega)$  and its Lorentzian square  $[L(\omega)]^2$  functions, where  $L(\omega) \propto \frac{\gamma^2}{4\pi(\Delta\omega^2 + \gamma^2)}$  and  $\omega$  is the angular frequency. For fitting, we use the non-linear least square algorithm, with  $\gamma$  and the proportional constant serving as fit parameters.

**Figure S2** demonstrates the Lorentzian fitting over few isolated modes where left and right panels represents data in linear and semi-logarithmic scales, respectively. The filled curves represent the experimental data, whereas the blue plots are  $L(\omega)$  fits, respectively. Clearly, every localized mode shows significantly better Lorentzian fit.

However, in the case of EPs (as illustrated in **Figure S3**), the Lorentzian curves significantly diverge from the experimental data in the decaying tails. In contrast, Lorentzian square fits  $[L(\omega)]^2$  provide significantly better fits, demonstrating increased output coupled intensity in EP modes and 2-fold degeneracy.

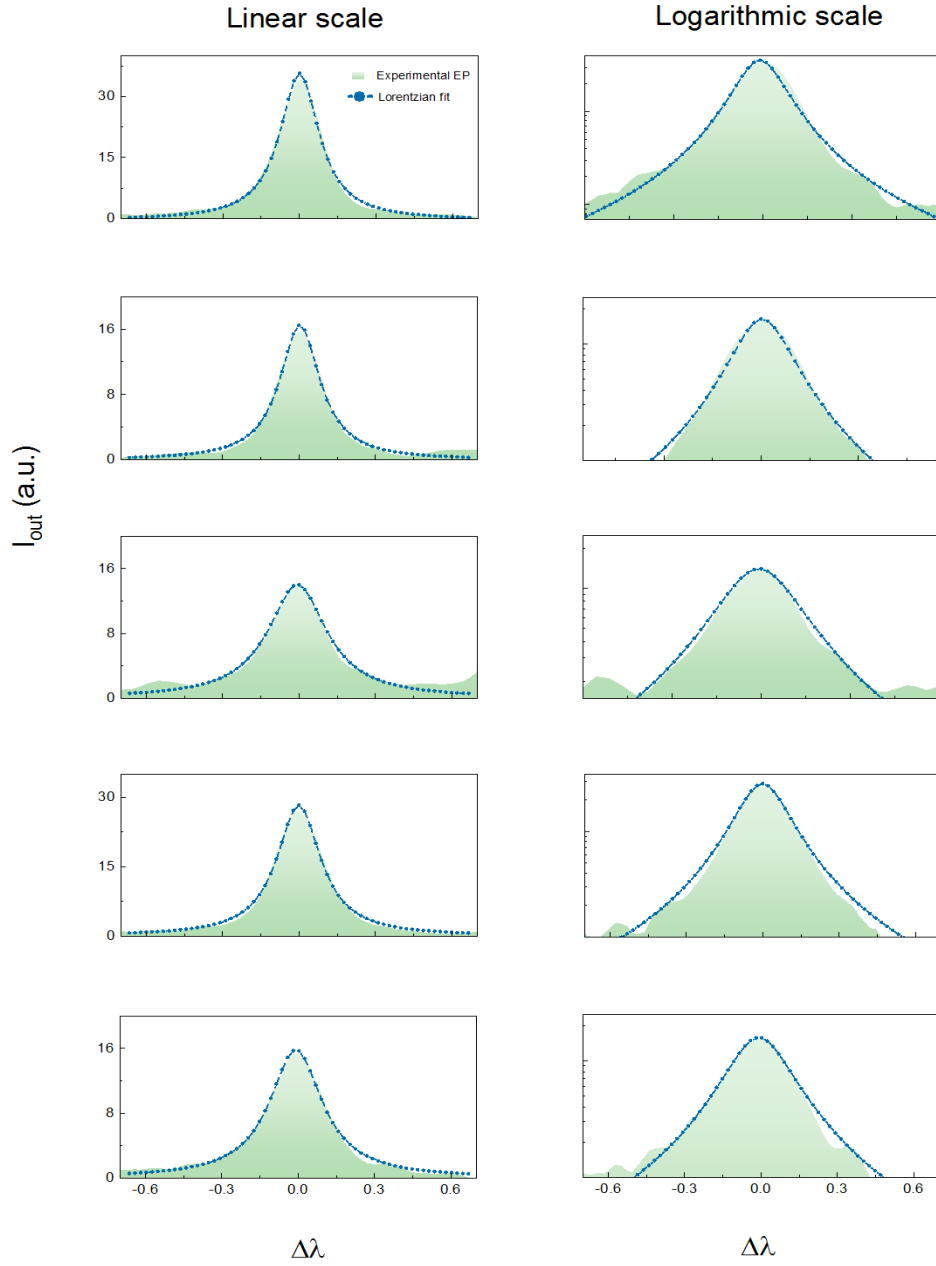

**Figure S2:** Spectral response of measured isolated **Anderson localized modes** and corresponding theoretical fits. Experimental data are represented by filled green plots. The blue plots are Lorentzian fits to the data. Left and right: linear and semi-logarithmic plots of the data, respectively.

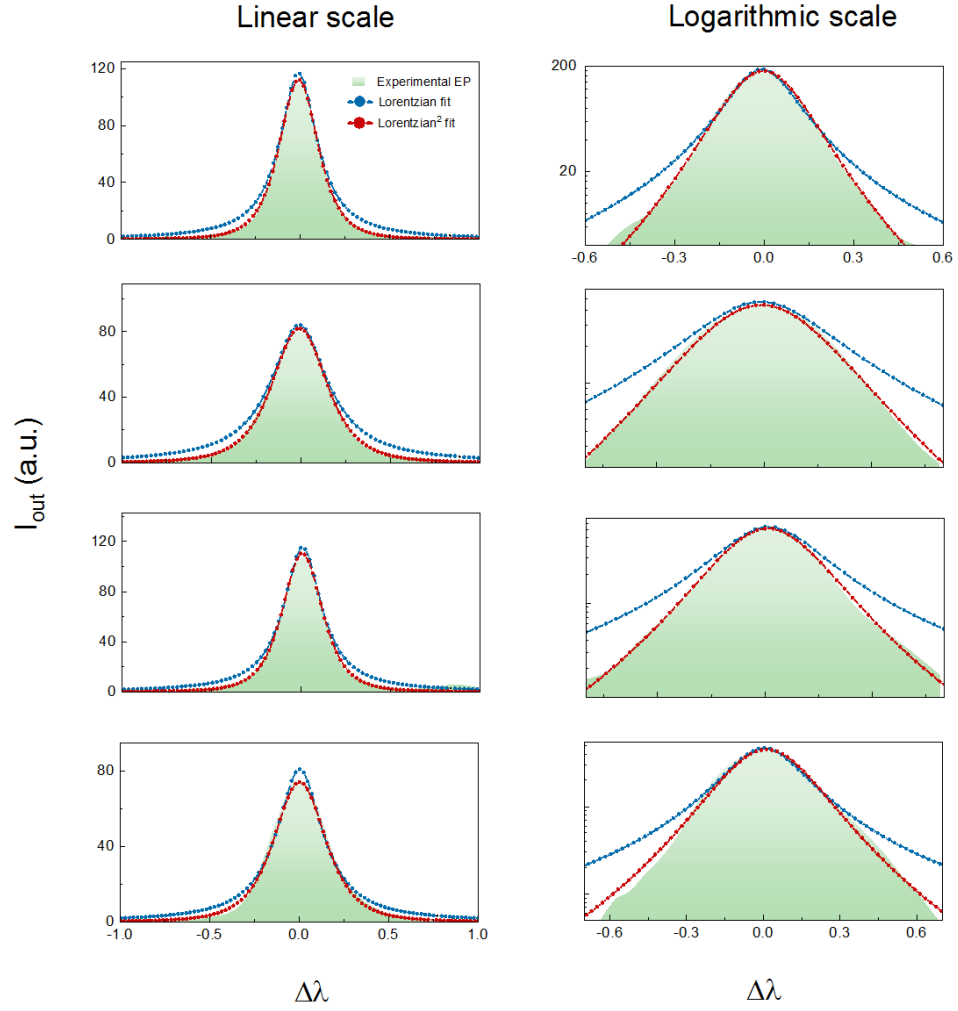

**Figure S3:** Spectral response of measured modes at **exceptional points (EPs)** and corresponding theoretical fits. Experiment data are represented by filled green plots. The blue and red plots are Lorentzian and Lorentzian square fits to the data, respectively.
